# Supplementary material for: Bi-Level Policy Optimization with Nystr\"om Hypergradients
Source: arXiv:2505.11714 source file (2026-03-17)
Supplement: Supplementary file 1 [file content.tex]

\makeatletter
\let\orig@pdfborder\@pdfborder
\makeatother

% Locally override for the appendix TOC
{
  \makeatletter
  \def\@pdfborder{0 0 0} % remove red boxes just here
  \makeatother

  \addtocontents{toc}{\protect\setcounter{tocdepth}{2}}
  
  \Large
  \tableofcontents
}

% Restore normal hyperlink behavior afterwards
\makeatletter
\let\@pdfborder\orig@pdfborder
\makeatother
